# Supplementary material for: Observation of a Transition Between Dynamical Phases in a Quantum Degenerate Fermi Gas
Source: arXiv:1806.11044 ancillary file (2019-03-05)
Supplement: Supplementary file 1 [file SMpaperV1.pdf]

# Supplementary Material for “Observation of a Dynamical Phase Transition in the Collective Heisenberg Model Simulated with Ultracold Fermions”

## CONTENTS

|                                                                            |    |
|----------------------------------------------------------------------------|----|
| I. Spin models                                                             | 1  |
| A. Effective Hamiltonian: Heisenberg model                                 | 1  |
| B. Scaling of the spin coupling parameters                                 | 2  |
| C. Mean-field model                                                        | 3  |
| II. Mean-field analytic solutions                                          | 3  |
| A. Lax vector analysis                                                     | 4  |
| B. Bloch equations analysis                                                | 6  |
| III. Beyond the spin-model approximation                                   | 8  |
| A. Non-interacting regime                                                  | 8  |
| B. Interacting regime                                                      | 9  |
| IV. Sample preparation and measurement                                     | 9  |
| A. Preparation                                                             | 9  |
| B. Measurement                                                             | 10 |
| C. Determining the zero-crossing of the $^{40}\text{K}$ Feshbach resonance | 10 |
| V. Data analysis for fine exploration of DPT (Figure 3)                    | 12 |
| VI. Scattering rate of the non-equilibrium gas                             | 14 |
| A. Equilibrium scattering rate                                             | 15 |
| B. Finite polarization, prepared out of equilibrium                        | 16 |
| References                                                                 | 18 |

## I. SPIN MODELS

### A. Effective Hamiltonian: Heisenberg model

In the experiment,  $N$  identical fermionic  $^{40}\text{K}$  atoms with mass  $m$  are trapped in a three dimensional spin-dependent nearly harmonic potential. The spin degree of freedom is encoded in the  $m_F = -9/2(\downarrow)$  and  $m_F = -7/2(\uparrow)$  states of the  $F = 9/2$  hyperfine manifold. The single-particle Hamiltonian of the system can be written as

$$\hat{H}_{\text{sp}} = \sum_{\sigma=\uparrow,\downarrow} \int d^3\mathbf{r} \hat{\psi}_{\sigma}^{\dagger}(\mathbf{r}) \left( -\frac{\hbar^2}{2m} \left( \frac{\partial^2}{\partial x^2} + \frac{\partial^2}{\partial y^2} + \frac{\partial^2}{\partial z^2} \right) + V_{\sigma}(\mathbf{r}) \right) \hat{\psi}_{\sigma}(\mathbf{r}), \quad (1)$$

where  $\hat{\psi}_{\sigma}^{\dagger}(\mathbf{r})$  is the fermionic field operator that creates a spin  $\sigma$  atom at point  $\mathbf{r}$ . For convenience we expand  $\hat{\psi}_{\sigma}^{\dagger}(\mathbf{r})$  in terms of fermionic operators  $\hat{c}_{\mathbf{n}\sigma}^{\dagger}$  that create a spin  $\sigma$  atom in the single particle eigenstate  $\phi_{\mathbf{n}}^{\sigma}(\mathbf{r})$  with  $\mathbf{n} = \{n_x, n_y, n_z\}$ . In this eigenmode basis the field operator takes the form

$$\hat{\psi}_{\sigma}^{\dagger}(\mathbf{r}) = \sum_{\mathbf{n}} \hat{c}_{\mathbf{n}\sigma}^{\dagger} \phi_{\mathbf{n}}^{\sigma}(\mathbf{r}). \quad (2)$$

The external potential can be written in the form of  $V_{\sigma}(\mathbf{r}) = V_0(\mathbf{r}) + \Delta V_{\sigma}(\mathbf{r})$ , where  $V_0(\mathbf{r})$  is the spin independent part of the potential with trapping frequencies  $\boldsymbol{\omega} = \{\omega_x, \omega_y, \omega_z\}$ . The term  $\Delta V_{\sigma}(\mathbf{r})$  describes the spin dependent part which naturally arises due to the slightly different magnetic moment between the two relevant internal states. The latter can be additionally tuned by polarization control (see Sec. IV).

In the eigenmode basis the single particle Hamiltonian simplifies to

$$\hat{H}_{\text{sp}} = \sum_{\mathbf{n}} \left( \left( \mathbf{n} + \frac{1}{2} \right) \cdot \hbar \boldsymbol{\omega} \hat{N}_{\mathbf{n}} + \left( \mathbf{n} + \frac{1}{2} \right) \cdot \hbar \Delta \boldsymbol{\omega} \hat{\sigma}_{\mathbf{n}}^Z \right), \quad (3)$$

where  $\hat{N}_{\mathbf{n}} = \hat{c}_{\mathbf{n}\uparrow}^\dagger \hat{c}_{\mathbf{n}\uparrow} + \hat{c}_{\mathbf{n}\downarrow}^\dagger \hat{c}_{\mathbf{n}\downarrow}$  and  $\{\hat{\sigma}_{\mathbf{n}}^X, \hat{\sigma}_{\mathbf{n}}^Y, \hat{\sigma}_{\mathbf{n}}^Z\} = \sum_{\alpha, \beta=\uparrow, \downarrow} \hat{c}_{\mathbf{n}\alpha}^\dagger \hat{\sigma}_{\alpha\beta} \hat{c}_{\mathbf{n}\beta}$  with  $\hat{\sigma}$  the vector of Pauli matrices.

Due to quantum statistics, spin polarized fermions cannot experience  $s$ -wave collisions. However, distinguishable fermions exhibit  $s$ -wave interactions described by the Hamiltonian

$$\hat{H}_{\text{int}} = \frac{4\pi\hbar^2 a}{m} \int d^3\mathbf{r} \hat{\rho}_{\uparrow}(\mathbf{r}) \hat{\rho}_{\downarrow}(\mathbf{r}), \quad (4)$$

where  $a$  is the  $s$ -wave scattering length and  $\hat{\rho}_{\sigma}(\mathbf{r}) = \hat{\psi}_{\sigma}^\dagger(\mathbf{r}) \hat{\psi}_{\sigma}(\mathbf{r})$  is the density operator of particles with spin  $\sigma$ . Substituting Eq. 2 into  $\hat{H}_{\text{int}}$  it becomes

$$\hat{H}_{\text{int}} = \frac{4\pi\hbar^2 a}{m a_x a_y a_z} \sum_{\mathbf{n}, \mathbf{m}, \mathbf{p}, \mathbf{q}} \mathcal{J}_{\mathbf{nmpq}} \hat{c}_{\mathbf{n}\uparrow}^\dagger \hat{c}_{\mathbf{m}\uparrow} \hat{c}_{\mathbf{p}\downarrow}^\dagger \hat{c}_{\mathbf{q}\downarrow}, \quad (5)$$

where  $a_{x,y,z} = \sqrt{\hbar/(m\omega_{x,y,z})}$  are the harmonic oscillator lengths along the principal trap axes. The coupling strength  $\mathcal{J}_{\mathbf{nmpq}}$  can be computed as

$$\mathcal{J}_{\mathbf{nmpq}} = \prod_{i=x,y,z} a_i \int d\mathbf{r}_i \phi_{\mathbf{n}_i}^\uparrow(\mathbf{r}_i) \phi_{\mathbf{m}_i}^\uparrow(\mathbf{r}_i) \phi_{\mathbf{p}_i}^\downarrow(\mathbf{r}_i) \phi_{\mathbf{q}_i}^\downarrow(\mathbf{r}_i). \quad (6)$$

The exact solution of this problem is numerically intractable even for 10 particles. However, in the weakly interacting regime and weak spin dependent potential ( $\Delta V_{\sigma}(\mathbf{r}) \ll V_0(\mathbf{r})$ ), it is possible to simplify the interaction Hamiltonian while still capturing the main physics, by making the key approximation that when particles collide, the single particle energy penalty to change modes after a collision suppresses mode changes. Under this picture the only relevant collisional processes that take place are those in which particles remain fixed in their modes. Colliding partners are however allowed to exchange their internal state. The two possible processes are:

- Spins remain the same:  $\mathbf{n} = \mathbf{m}$ ,  $\mathbf{p} = \mathbf{q}$ ,  $\mathcal{J}_{ij}^z = \mathcal{J}_{ijjj}$
- Spins flip:  $\mathbf{n} = \mathbf{q}$ ,  $\mathbf{m} = \mathbf{p}$ ,  $\mathcal{J}_{ij}^\perp = \mathcal{J}_{ijji}$ ,

where  $i, j$  are indices of the eigenmodes of the single-particle Hamiltonian. For current experimental conditions,  $\Delta\omega_i/\omega_i \ll 1$ , the single-particle wavefunctions for the two spin states are approximately the same and therefore  $\mathcal{J}_{ij} \equiv \mathcal{J}_{ij}^\perp \approx \mathcal{J}_{ij}^z$ . Consequently the interaction Hamiltonian remains SU(2) invariant, and it is described by a collective Heisenberg spin model:

$$\hat{H}_{\text{int}}/\hbar \approx -\frac{1}{4} \sum_{ij} J_{ij} \hat{\sigma}_i \cdot \hat{\sigma}_j = -\sum_{ij} J_{ij} \hat{\mathbf{s}}_i \cdot \hat{\mathbf{s}}_j, \quad (7)$$

where  $\hat{\mathbf{s}} = \frac{1}{2} \hat{\sigma}$  are spin-1/2 operators. We have written the spin coupling amplitudes as  $J_{ij} = U \mathcal{J}_{ij}$  with  $U = 4\pi\hbar a/(m a_x a_y a_z)$ .

Since in this frozen-motion approximation,  $\hat{N}_{\mathbf{n}}$  remains a constant, the first term in Eq. (3) can be dropped from the Hamiltonian. The total Hamiltonian thus takes the form of a Heisenberg spin model plus an additional inhomogeneous transverse field:

$$\hat{H}/\hbar = \sum_i h_i \hat{s}_i^Z - \sum_{ij} J_{ij} \hat{\mathbf{s}}_i \cdot \hat{\mathbf{s}}_j, \quad (8)$$

where  $i, j$  run over the occupied modes and  $h_i = 2\mathbf{n}_i \cdot \Delta\boldsymbol{\omega}$  is the differential local field experienced by an atom in the  $i$ th mode.

## B. Scaling of the spin coupling parameters

The coupling terms  $\mathcal{J}_{\mathbf{nmmn}}$  involve integrals of the square of two different harmonic oscillator modes, and thus can mimic long-range interactions. In fact, the integrals can be shown to asymptotically scale as  $\sim 1/\sqrt{|n_p - m_p|}$  in

each direction. This scaling can be used to approximately estimate the mean value  $\mathcal{J} = 1/N^2 \sum_{i,j} \mathcal{J}_{ij}$ :

$$\begin{aligned} \mathcal{J} &\propto \frac{1}{N^2} \prod_{p=x,y,z} \left( \sum_{n_p, m_p}^{N_p} \frac{1}{\sqrt{|n_p - m_p|}} \right) \\ &\propto \frac{1}{N^2} \prod_{p=x,y,z} \left( \int_0^{N_p} dn_p \int_0^{N_p} dm_p \frac{1}{\sqrt{|n_p - m_p|}} \right) \\ &\propto \frac{1}{N^2} (N_x N_y N_z)^{3/2} = N^{-\frac{1}{2}}. \end{aligned} \quad (9)$$

with  $N = N_x N_y N_z$ , and  $N_{x,y,z}$  are the harmonic oscillator quantum numbers associated with the Fermi level along each trap direction.

### C. Mean-field model

To calculate the many-body dynamics of  $\hat{H}_{\text{int}}$  we use a mean-field approximation which neglects quantum correlations between different particles, namely  $\langle \hat{s}_i^p \hat{s}_j^{p'} \rangle \approx \langle \hat{s}_i^p \rangle \langle \hat{s}_j^{p'} \rangle$ . Under this assumption the interacting Hamiltonian can be written as a non-linear single particle Hamiltonian of the form  $\hat{H}_{\text{mf}} = \sum_j \hat{H}_{\text{mf}}^{(j)}$ , where the sum runs over all occupied single particle modes. The Hamiltonian felt by the  $j$ th particle corresponds to an effective self-adjusting magnetic field generated by its interaction with all other particles in the array. Explicitly,

$$\hat{H}_{\text{mf}}^{(j)} / \hbar = \hat{\mathbf{s}}_j \cdot \mathbf{B}_j. \quad (10)$$

where  $\mathbf{B}_j = (-2 \sum_i J_{ij} s_i^X, -2 \sum_i J_{ij} s_i^Y, -2 \sum_i J_{ij} s_i^Z + h_j)$  with  $\mathbf{s}_i = \langle \hat{\mathbf{s}}_i \rangle$  and  $s_i^\pm = \langle \hat{s}_i^\pm \rangle$ . Accordingly, the non-linear equations are given by

$$\begin{aligned} i \frac{ds_j^+}{dt} &= 2 \left( s_j^Z \sum_k J_{kj} s_k^+ - s_j^+ \sum_k J_{kj} s_k^Z \right) + h_j s_j^+ \\ i \frac{ds_j^-}{dt} &= -2 \left( s_j^Z \sum_k J_{kj} s_k^- - s_j^- \sum_k J_{kj} s_k^Z \right) - h_j s_j^- \\ i \frac{ds_j^Z}{dt} &= s_j^+ \sum_k J_{kj} s_k^- - s_j^- \sum_k J_{kj} s_k^+. \end{aligned} \quad (11)$$

All numerical solutions in the main text are obtained by numerically solving Eq. (11). On the timescales probed by the experiment, we see good agreement between the mean-field simulation, which ignores correlations, with exact solutions which include quantum correlations, confirming the validity of the mean-field model.

Due to the large number of particles ( $N \sim 10^4$ ), a full mean-field model would involve solving  $\sim 10^5$  differential equations, which would be extremely slow. Instead, we solve a smaller system with  $N_0 \sim 10^3$  and exploit the scaling of  $J_{ij}$  and  $\hbar^2$  with particle number to reproduce the large- $N$  dynamics. Specifically in the small- $N_0$  simulation, we scale  $J_{ij} \rightarrow J_{ij}(N/N_0)^{1/2}$  and  $h_i \rightarrow h_i(N/N_0)^{1/3}$  to match the corresponding parameters of the large system.

## II. MEAN-FIELD ANALYTIC SOLUTIONS

Even at the mean-field level, an analytic solution of the non-linear dynamics dictated by Eq. (11) is not simple due to the inhomogeneity of the coupling coefficients  $J_{ij}$ . The long-range character of the couplings discussed in Sec. IB further allows us to approximately replace the inhomogeneous  $J_{ij}$  by an effective all-to-all coupling parameter  $J$ . Under this approximation, the Hamiltonian Eq. (8) can be written in terms of the collective spin operators  $\hat{\mathbf{S}} = \sum_i \hat{\mathbf{s}}_i$  as

$$\hat{H} / \hbar \approx \sum_i h_i \hat{s}_i^Z - J \hat{\mathbf{S}} \cdot \hat{\mathbf{S}}. \quad (12)$$

In this section, we use two approaches to derive mean-field analytic expressions of the dynamics of Eq. 12. Both solutions qualitatively capture the behavior of Eq. 8, and they provide complementary insight into the underlying

physics.

### A. Lax vector analysis

Many of the features observed in our system can be understood based on the underlying integrability of the fully connected Heisenberg model, such as the nature of the two dynamical phases, the non-analytical scaling of the order parameter (see Fig. 3G) and of the oscillation frequency of the dynamical ferromagnet (see Fig. 3H) close to the non-equilibrium critical point. This analysis parallels the techniques of Refs. [1–3] for the non-equilibrium quench dynamics of BCS-type models, which are formally equivalent to the spin model with homogeneous spin-spin interactions, Eq. 12, in Anderson’s pseudo-spin representation. In the BCS models, the  $\hat{S}^Z \hat{S}^Z$  component of the interactions is not present. However, since this term reduces to  $2\hat{S}^Z \langle \hat{S}^Z \rangle$  at the mean-field level, it can be rotated out. Furthermore, for our initial conditions  $\langle \hat{S}^Z \rangle = 0$ , the term exactly vanishes, making the models identical.

Fully connected models such as Eq. 12 admit an exact solution. Its underlying *classical* integrability allows for an exact determination of the frequency spectrum ruling non-equilibrium dynamics. We introduce the *Lax vector*,  $\mathbf{L}(u)$ , of the complex-valued auxiliary variable  $u$ , associated with the Hamiltonian of Eq. 12,

$$\mathbf{L}(u) \equiv \sum_{j=1}^N \frac{\mathbf{s}_j}{u - h_j/2} - \frac{\mathbf{Z}}{J}, \quad (13)$$

along the lines of Refs. [1–3]. The squared Lax vector  $L^2(u)$  is an integral of motion, and can be therefore evaluated for convenience at time  $t = 0$ : it is fixed by the initial non-equilibrium condition. Starting with a spin state fully polarized along the  $X$ -direction gives

$$L_X(u) = \frac{1}{2} \sum_{i=1}^N \frac{1}{u - h_i/2}, \quad L_Y(u) = 0, \quad L_Z(u) = -\frac{1}{J}. \quad (14)$$

The  $2N$  roots (coming in complex conjugate pairs) of  $L^2(u) = 0$  are the eigenfrequencies governing the dynamics of the model; the order parameter  $\mathcal{S}^+(t)$  will exhibit oscillatory behavior with frequencies corresponding to these roots. The locations of the roots in the complex plane also indicate whether the expectation value  $\mathcal{S}^+(t) = \sum_i \langle \hat{s}_i^+(t) \rangle$  relaxes towards zero (demagnetized phase) or towards a non-zero value (dynamical ferromagnetic phase). The demagnetized phase results when all  $2N$  roots are in the neighborhood of the real axis, since destructive interference among the different oscillating modes will cause inhomogeneous dephasing. In the dynamical ferromagnetic phase of Eq. 12, we find two complex conjugate roots separated from the other  $2N - 2$  roots along the real axis, leading to non-vanishing  $\mathcal{S}(\infty) = |\mathcal{S}^+(\infty)|$ .

In a 1D system with an axial field of the form  $h_i/2 = (i - N/2)\Delta\omega$ , the inhomogeneity is  $\tilde{h} = N\Delta\omega/\sqrt{3}$ . In the

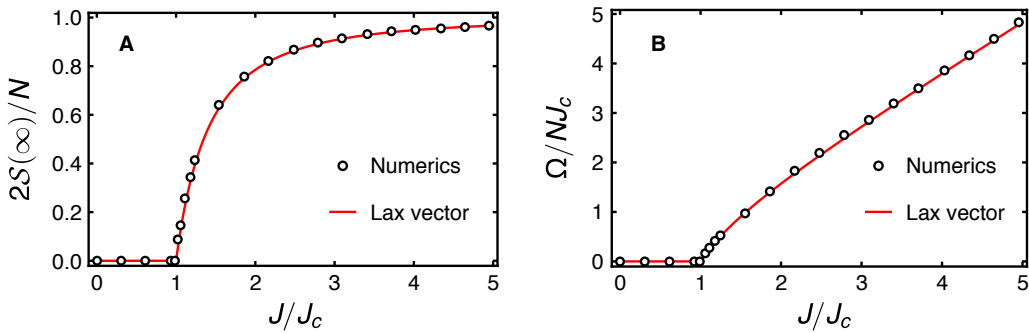

FIG. 1. Comparison between numerical solution of the non-linear mean-field equations and the analytic Lax vector results (Eqs. 16, 17) for the collective model (Eq. 10). (A) shows the steady state magnetization  $|\mathcal{S}_+(\infty)| = \mathcal{S}(\infty)$ , and (B) shows its transient oscillation frequency  $\Omega$ .

large- $N$  limit, the summation in  $L_X(u)$  can be approximated by an integral, namely

$$L_X(u) \approx \frac{1}{2\Delta\omega} \int_{-N/2}^{N/2} \frac{d\zeta}{u/\Delta\omega - \zeta} = \frac{1}{2\Delta\omega} \ln \left( \frac{u/\Delta\omega + N/2}{u/\Delta\omega - N/2} \right). \quad (15)$$

The imaginary part of this expression ranges from 0 to  $\pi/(2\Delta\omega)$ , so roots of  $L^2(u) = 0$  will exist only if  $1/J \leq \pi/(2\Delta\omega) = N\pi/(2\sqrt{3}\tilde{h})$ . For  $J < J_c \equiv 2\sqrt{3}\tilde{h}/N\pi$ ,  $\mathcal{S}^+(t)$  relaxes towards a stationary zero value with zero oscillation frequency (demagnetized phase). For  $J \geq J_c$ , the two complex conjugate roots are given by

$$u = \pm i\Omega/2 = \pm i \frac{\sqrt{3}\tilde{h}}{2} \cot \left( \frac{\sqrt{3}\tilde{h}}{NJ} \right) = \pm i \frac{N\pi J_c}{4} \cot \left( \frac{\pi J_c}{2J} \right). \quad (16)$$

Accordingly, the steady-state order parameter in this ferromagnetic phase approaches its steady state as [3]:

$$\mathcal{S}(t) \rightarrow \mathcal{S}(\infty) \left( 1 + \frac{A}{\sqrt{\Omega t}} \cos(\Omega t + \Phi_A) \right), \quad (17)$$

with  $A$  and  $\Phi_A$  constants set by the system parameters and initial conditions, and

$$\mathcal{S}(\infty) = \left| \frac{u}{J} \right| = \frac{\sqrt{3}\tilde{h}}{2J} \cot \left( \frac{\sqrt{3}\tilde{h}}{NJ} \right) = \frac{N\pi J_c}{4J} \cot \left( \frac{\pi J_c}{2J} \right). \quad (18)$$

The oscillation frequency  $\Omega$  and steady-state magnetization  $\mathcal{S}(\infty)$  can also be obtained by numerically solving the Bloch equations (Eq. 11). The solutions agree with the analytic expression of Eqs. 16, 17 as shown in Fig. 1.

Even though generalization of the Lax vector method to higher dimensions with axial field  $h_i = 2\mathbf{n}_i \cdot \Delta\boldsymbol{\omega}$  is straightforward, concise analytic expressions of the roots  $u$  are not accessible, so we find them numerically. To satisfy  $L^2(u) = 0$ , we need to find a pair of complex conjugate numbers  $u = u_{\text{Re}} \pm iu_{\text{Im}}$  for which  $L_X(u)$  is purely imaginary, hence for each  $u_{\text{Im}}$ , there is a unique  $u_{\text{Re}}$  (see Fig. 2).  $u_{\text{Re}}$  represents the global precession rate of  $\mathcal{S}_+(t)$  and  $u_{\text{Im}}$  represents oscillation rate of  $\mathcal{S}(t)$ .

As shown in Fig. 2,  $L_X(u)$  can be approximated by

$$L_X(u) \approx i \frac{N}{2\sqrt{3}\alpha\tilde{h}} \ln \left( \frac{i u_{\text{Im}} + \sqrt{3}\alpha\tilde{h}/2}{i u_{\text{Im}} - \sqrt{3}\alpha\tilde{h}/2} \right), \quad (19)$$

where  $\alpha$  is a dimensionless constant that depends on the distribution of  $h_i$ . Using this approximation, similar to the

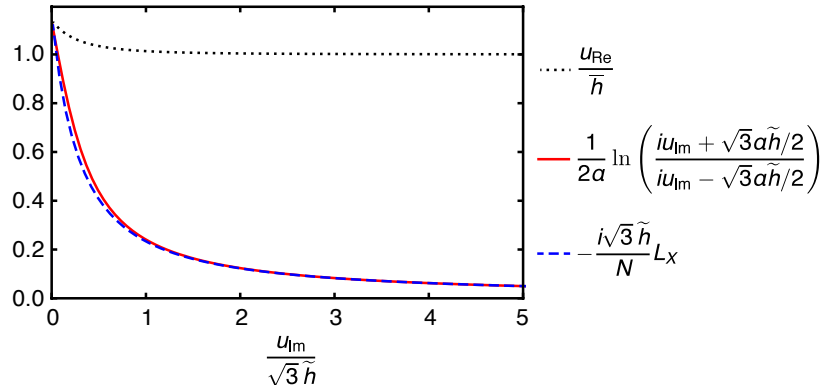

FIG. 2. A 3D system with axial fields  $h_i = 2\mathbf{n}_i \cdot \Delta\boldsymbol{\omega}$  where  $\Delta\omega_x = 0.9\Delta\omega_y = 0.8\Delta\omega_z$ , with mean value  $\bar{h}$  and standard deviation  $\tilde{h}$ . In order to satisfy  $L^2(u) = 0$ ,  $L_X(u)$  must be a pure imaginary number, hence for each  $u_{\text{Im}}$ , there is one associated  $u_{\text{Re}}$  that satisfies this condition. The plot shows how  $L_X(u)$  (dashed blue line) and  $u_{\text{Re}}$  (dotted black line) vary with  $u_{\text{Im}}$ .  $L_X(u)$  approximately takes the form of Eq. (19) with  $\alpha = 1.39$  for this set of  $h_i$  (solid red line).

1D case, we find the parameters that admit a pair of complex roots. For  $J < J_c \equiv 2\sqrt{3}\alpha\tilde{h}/N\pi$ , there are no roots, but for  $J > J_c$ ,  $u_{\text{Im}}$  has a finite value given by

$$u_{\text{Im}} = \pm\Omega/2 = \pm\frac{\sqrt{3}\alpha\tilde{h}}{2}\cot\left(\frac{\sqrt{3}\alpha\tilde{h}}{NJ}\right), \quad \mathcal{S}(\infty) = \left|\frac{u_{\text{Im}}}{J}\right| = \frac{\sqrt{3}\alpha\tilde{h}}{2J}\cot\left(\frac{\sqrt{3}\alpha\tilde{h}}{NJ}\right). \quad (20)$$

We also numerically find that the long time dynamics in the 3D system is well described by the same asymptotic behavior exhibited by the 1D case:

$$\mathcal{S}(t) \rightarrow \mathcal{S}(\infty) \left(1 + \frac{B}{\sqrt{\Omega t}} \cos(\Omega t + \Phi_B)\right), \quad (21)$$

where  $B$  and  $\Phi_B$  are constants determined by system parameters.

The above derivation is based on all-to-all couplings  $J_{ij} = J$ . To account for non-collective interactions, we introduce another renormalization parameter  $J_{\text{eff}} = \beta J$  leading to

$$u_{\text{Im}} = \pm\frac{\sqrt{3}\alpha\tilde{h}}{2}\cot\left(\frac{\sqrt{3}\alpha\tilde{h}}{NJ_{\text{eff}}}\right), \quad \mathcal{S}(\infty) = \left|\frac{u_{\text{Im}}}{J_{\text{eff}}}\right| = \frac{\sqrt{3}\alpha\tilde{h}}{2J_{\text{eff}}}\cot\left(\frac{\sqrt{3}\alpha\tilde{h}}{NJ_{\text{eff}}}\right). \quad (22)$$

## B. Bloch equations analysis

For the all-to-all coupling case, the effective magnetic field simplifies to  $\mathbf{B}_j = \{-2JS^X, -2JS^Y, -2JS^Z + h_j\}$  with  $\mathbf{S} = \sum_i \langle \hat{\mathbf{s}}_i \rangle$ . First we note that  $\hat{S}^Z$  commutes with the Hamiltonian so  $S^Z$  remains constant during the dynamics. The initial  $\pi/2$ -pulse used to induce dynamics in our experiment generates a system initially polarized along  $X$ , so  $S^Z = 0$ . The resulting non-linear Bloch equations obtained from the mean-field Hamiltonian are

$$\begin{aligned} \frac{ds_j^+}{dt} &= -2iJs_j^Z S^+ - ih_js_j^+ \\ \frac{ds_j^Z}{dt} &= -iJ(s_j^+ S^- - s_j^- S^+). \end{aligned} \quad (23)$$

These equations of motion can be rewritten in terms of the spin collective observables  $\mathcal{S}^{\pm,Z}$  and the  $h$ -weighted spin-wave variables  $\mathcal{C}^{\pm,Z} = \sum_j (h_j - \bar{h}) s_j^{\pm,Z} / \tilde{h}$  ( $\bar{h} = \sum_i h_i / N$  and  $\tilde{h} = \sqrt{\sum_i h_i^2 / N - \bar{h}^2}$ ) as

$$\begin{aligned} \frac{d\mathcal{S}^+}{dt} &= -i\tilde{h}\mathcal{C}^+ - i\bar{h}\mathcal{S}^+ \\ \frac{d\mathcal{C}^+}{dt} &= -2iJ\mathcal{C}^Z \mathcal{S}^+ - i\sum (h_j - \bar{h})^2 s_j^+ / \tilde{h} - i\bar{h}\mathcal{C}^+ \\ \frac{d\mathcal{C}^Z}{dt} &= -iJ(\mathcal{C}^+ \mathcal{S}^- - \mathcal{C}^- \mathcal{S}^+). \end{aligned} \quad (24)$$

In the gap-protected regime, the particles are expected to be phase-locked, and it is reasonable to assume that  $s_i^+ = \mathcal{S}^+ / N$ . In the rotation frame  $\bar{h} = 0$ , together with the approximation that  $\text{Re}(\mathcal{C}^+ \mathcal{S}^-) \approx 0$ , which we confirm numerically, we obtain a set of closed equations

$$\frac{d^2 \mathcal{S}^+}{dt^2} \approx -2\tilde{h}\mathcal{C}^Z \mathcal{S}^+ - \tilde{h}^2 \mathcal{S}^+ \quad (25a)$$

$$\frac{d^2 \mathcal{C}^+}{dt^2} \approx -\Omega^2 \mathcal{C}^+ - 2\tilde{h}\mathcal{C}^Z \mathcal{C}^+ - \tilde{h}^2 \mathcal{C}^+, \quad (25b)$$

where we define  $\Omega = 2J|\mathcal{S}^+|$ . In the large interaction limit,  $JN/\tilde{h} \gg 1$ , neglecting terms proportional to  $\tilde{h}$  yields simple second order differential equations for  $\mathcal{C}_{(0)}^+$  and  $\mathcal{S}_{(0)}^+$ :

$$\frac{d^2 \mathcal{C}_{(0)}^+}{dt^2} \approx -\Omega_{(0)}^2 \mathcal{C}_{(0)}^+ \quad \frac{d^2 \mathcal{S}_{(0)}^+}{dt^2} \approx 0, \quad (26a)$$

from which we obtain  $\mathcal{S}_{(0)}^+ \approx N/2$  and  $\Omega_{(0)} \approx NJ$ . The mean field energy  $\hbar\Omega_{(0)}$  matches the energy splitting between the  $S = N/2$  Dicke states and the  $S = N/2 - 1$  states in the quantum model ( $\hbar J \hat{\mathbf{S}} \cdot \hat{\mathbf{S}}$ ). Similar to the quantum case, this energy gap is responsible for the robustness of the initial coherent state to dephasing in the mean-field model.

Including corrections of order  $\tilde{\hbar}$  and substituting Eq. 27 into Eq. 25a, together with the energy conservation constraint

$$\tilde{\hbar}\mathcal{C}^Z = J(|\mathcal{S}^+|^2 - N^2/4), \quad (27)$$

we obtain

$$\frac{d^2 \mathcal{S}_{(1)}^+}{dt^2} = -J^2 \mathcal{S}_{(1)}^+ \left( 4|\mathcal{S}_{(1)}^+|^2 - N^2 \right) / 2 - \tilde{\hbar}^2 \mathcal{S}_{(1)}^+ \equiv -\frac{\partial V(\mathcal{S}_{(1)}^+)}{\partial \mathcal{S}_{(1)}^+}. \quad (28)$$

Eq. (28) describes the motion of a particle with the generalized coordinate  $\mathcal{S}_{(1)}^+$  in the potential  $V(\mathcal{S}_{(1)}^+)$  given by

$$V(\mathcal{S}_{(1)}^+) = \frac{1}{4}J^2 \left( \mathcal{S}_{(1)}^+ \right)^4 + \frac{1}{2} \left( \tilde{\hbar}^2 - N^2 J^2 / 2 \right) \left( \mathcal{S}_{(1)}^+ \right)^2. \quad (29)$$

The potential written as a function of the order parameter  $\mathcal{S}^+$  has the characteristic form of the Landau free energy functional which is often called the “wine bottle” or “Mexican hat” potential, and it describes second-order phase transitions. For  $\tilde{\hbar} > NJ/\sqrt{2}$  it admits a single minimum at  $\mathcal{S}^+ = 0$ , which describes the demagnetized disorder phase. In contrast, for  $\tilde{\hbar} < NJ/\sqrt{2}$ , the potential develops a non-trivial minimum, implying finite magnetization and signaling the development of a broken symmetry. The classical analog corresponds to the case where the system rolls to the bottom of the wine bottle (see Fig. 3). This Landau-Ginzburg picture has been postulated in field theoretical approaches to dynamical phase transitions [4–6], and Eq. 29 confirms that this is the appropriate emergent structure starting from the microscopic model Eq. 12. In the steady state, the particle rests at the potential minimum, yielding

$$|\mathcal{S}_{(1)}^+(\infty)| = \begin{cases} \frac{1}{2}\sqrt{N^2 - 2\tilde{\hbar}^2/J^2}, & \text{if } NJ \geq \sqrt{2}\tilde{\hbar} \\ 0, & \text{if } NJ < \sqrt{2}\tilde{\hbar}. \end{cases} \quad (30)$$

The dynamical behavior in the two phases is qualitatively different. For  $NJ \ll \sqrt{2}\tilde{\hbar}$ , the magnetization drops quickly without oscillations due to dephasing. In the limit  $NJ \gg \sqrt{2}\tilde{\hbar}$ , the potential in the vicinity around  $\mathcal{S}_{(1)}^+(\infty)$  is nearly

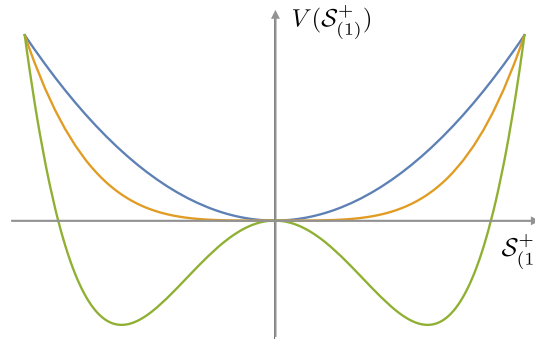

FIG. 3. Effective mean field potential (Eq. (29)):  $NJ = 0$  (blue): purely harmonic potential, with a minimum at  $\mathcal{S}_{(1)}^+(\infty) = 0$ ;  $NJ = \sqrt{2}\tilde{\hbar}$  (yellow): critical point, the potential become purely quartic. For  $NJ > \sqrt{2}\tilde{\hbar}$  (green) the trivial case  $\mathcal{S}_{(1)}^+(\infty) = 0$  is no longer a stable steady state and the potential exhibits the characteristic Mexican hat shape with minima at  $|\mathcal{S}_{(1)}^+(\infty)| > 0$ .

harmonic,  $V(\mathcal{S}_{(1)}^+) \approx \frac{1}{2}\Omega_{(1)}^2(\mathcal{S}_{(1)}^+)^2$ , exhibiting oscillations with frequency  $\Omega_{(1)}$

$$\Omega_{(1)} = \sqrt{\left. \frac{\partial^2 V(\mathcal{S}_{(1)}^+)}{\partial^2 \mathcal{S}_{(1)}^+} \right|_{\mathcal{S}_{(1)}^+ \rightarrow \mathcal{S}_{(1)}^+(\infty)}} = \sqrt{(NJ)^2 - 2\tilde{h}^2} \approx NJ - \frac{\tilde{h}^2}{NJ}. \quad (31)$$

The neglected higher order terms lead to slow damping of those oscillations in the steady state.

In contrast to the Lax vector method where an analytic formula for the roots of  $L^2(u) = 0$  is often not tractable for generic  $h_i$  distributions, Eqs. 30, 31 are general and simple since they only depend on  $\tilde{h}$ . On the other hand, they are only valid for  $NJ \gg \tilde{h}$ , as confirmed by comparison between the analytic expressions and numerical solutions. For  $NJ \ll \tilde{h}$ , Eqs. 30, 31 are only approximate, and their quantitative agreement largely depends on the distribution of  $h_j$ . For example, if  $h_i$  are drawn from a 1D cosine distribution, Eqs. 30, 31 become exact.

### III. BEYOND THE SPIN-MODEL APPROXIMATION

#### A. Non-interacting regime

In the experiment, atoms are trapped in a harmonic potential as well as a magnetic field gradient ( $V \propto \Delta\mathcal{B} \cdot \mathbf{r}\hat{\sigma}_z$ ). This combination leads to periodic spin-dependent displacements of the cloud: the spin components oscillate in opposite directions, leading to modulation of the magnetization at the same frequency. The atoms also experience a spin-dependent harmonic potential ( $V \propto \sum_{p=x,y,z} \Delta\omega_p p^2 \hat{\sigma}_z$ ) due to magnetic field curvature. In the presence of this additional spin-dependent harmonic potential, oscillations due to  $\Delta\mathcal{B}$  will decay at longer time due to the dephasing induced by  $\Delta\omega$ . In the spin model Hamiltonian Eq. 8, the effect of  $\Delta\omega$  is incorporated as  $\sum_i h_i \hat{s}_i^Z$  while the spin-dependent displacement is ignored. Under this simplification, the magnetization dynamics at zero interaction is given by

$$\mathcal{S}(t) = \frac{1}{2} \left| \sum_j e^{-ih_j t} \right|. \quad (32)$$

The comparison between this analytic expression and numerical simulations, which incorporate both effects, validates the spin model treatment of the dynamics (see Fig. 4). Since the amplitude of fast oscillations damps out for  $t > 30$  ms with typical experimental parameters, it is fairly reasonable to neglect them.

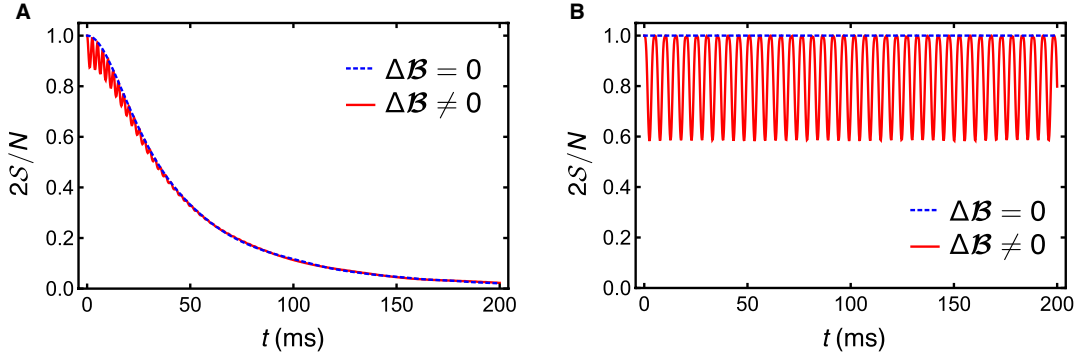

FIG. 4. Magnetization dynamics for non-interacting particles: (A) shows a comparison between the analytic expression based on the spin model dynamics (dashed blue line) and the non-interacting numerical calculations (solid red line) that include both a field gradient ( $\propto \Delta\mathcal{B}$ ) and a field curvature ( $\propto \Delta\omega$ ) in the Hamiltonian. (B) As in A, but with an additional spin-reversal pulse at the middle of the evolution. The pulse suppresses the dephasing (as seen by the constant level of the dashed blue line in B) but enhances the amplitude of the oscillation (solid red line). Parameters:  $N = 3.0 \times 10^4$  degenerate particles,  $k_B T = 0.3 E_F$ ,  $a_s = 0$ ,  $\Delta\omega_x/2\pi = 0.100$  Hz,  $\Delta\omega_y/2\pi = 0.043$  Hz,  $\Delta\omega_z/2\pi = 0.052$  Hz.

With the addition of a spin-reversal pulse at the middle of the evolution, the magnetization decay due to  $\Delta\omega$  is fully reversed, consistent with the spin model prediction. However, the amplitude of the differential center of mass oscillations of the two spin components due to  $\Delta\mathcal{B}$  is increased by a factor of two (see Ref. [7]), increasing in

turn the amplitude of the magnetization oscillations. The oscillatory behavior at zero interactions is not captured by the spin model and is a source of irreversibility in the non-interacting regime. We account for these processes in our theoretical simulations as an overall noisy background which decreases the amplitude of the magnetization. Roughly speaking, we multiply by an extra dephasing term  $e^{-\Gamma_0 t}$  in Fig. 4 where the time is set to  $t = 100$  ms and let  $\Gamma_0$  be a fitting parameter.

Since single-particle dephasing is different during evolution with a spin-reversal, we fit those data with a higher value of  $\Gamma_0$ , consistent with the increased amplitude of oscillations seen in Fig. 4.

## B. Interacting regime

Mode-changing collisions, which are not included in the spin model, also lead to magnetization decay. We account for them phenomenologically by adding an additional collisional dephasing term in the spin model, leading to exponential decay of the magnetization at a rate  $\Gamma = \Gamma_0 + (a/a_0)^2 \gamma$ . Here  $a_0$  is the Bohr radius, and the parameters  $\Gamma_0$  and  $\gamma$  are determined from fits to experimental data. The fitted  $\gamma$  is consistent with the expected depolarization rate generated by mode-changing collisions (see Sec. VI).

# IV. SAMPLE PREPARATION AND MEASUREMENT

## A. Preparation

We sympathetically cool fermionic spin-polarized  $^{40}\text{K}$  using bosonic  $^{87}\text{Rb}$ . Initially both species are trapped in the magnetic field produced by a microfabricated chip trap where  $^{87}\text{Rb}$  undergoes forced rf evaporative cooling. Subsequently both species are loaded into a crossed-beam optical dipole trap (ODT) with aspect ratio 6:1:1, followed by a final stage of evaporative cooling. A resonant light pulse removes any remaining  $^{87}\text{Rb}$  leaving a spin-polarized degenerate Fermi gas, typically with  $N = 4 \times 10^4$  atoms at a temperature  $T = 150$  nK in the lowest hyperfine level of the electronic ground state. We measure the temperature with time-of-flight imaging, and control it by varying the endpoint for trap beam power in the evaporation sequence. Optical trap frequencies during dynamics are  $\omega = 2\pi \times \{395, 1140, 950\}$  Hz. These are calibrated (with  $\lesssim 3\%$  accuracy) by following center-of-mass cloud displacement versus time after a step in cloud position.

We control the magnetic field and its gradients using a combination of macroscopic coils and wires on the atom chip  $\approx 200$   $\mu\text{m}$  from the atoms. We calibrate the field by measuring the  $|\downarrow\rangle$  to  $|\uparrow\rangle$  transition frequency and converting the frequency to magnetic field using the Breit-Rabi relation. During a measurement the field drifts by as much as 10 mG.

Magnetic field gradients are measured by repeating rf spectroscopy at various ODT trap displacements. We minimize the field gradients using microfabricated conductors near the trapped cloud. In the optimal configuration, gradients are  $\{1.3(1), 1.2(1), 0.2(5)\}$  G/cm. The displacements  $\Delta_i$  of the cloud that result from these gradients can be compared to the harmonic oscillator length  $a_i^2 = \hbar/m\omega_i$ , resulting in dimensionless displacements  $\Delta_i/a_i = \{2.1, 0.4, 0.1\} \times 10^{-2}$ .

The effective axial field  $h_i$  in the Heisenberg Hamiltonian comes from the inhomogeneous average field sampled by different motional eigenstates of the trap. The leading-order contribution to  $h_i$  is magnetic field curvature in real space. Using the data taken for magnetic field gradient calibration, the magnetic field curvatures can only be bounded to be  $\lesssim 500$  G/cm. Best-fit values from comparison to mean-field theory are field curvatures of  $\{200, 250, 250\}$  G/cm<sup>2</sup>.

We additionally control the inhomogeneity  $\tilde{h}$  by modifying the trap potential in a spin-dependent manner using the ODT light. For light with large detuning  $\delta$  from the atomic resonance frequency  $\omega_0$  and intensity profile  $I(\mathbf{r})$ , the potential experienced by the atoms is

$$U(\mathbf{r}) = \frac{3\pi c^2 \Gamma}{2\omega_0^2 \delta} \left( 1 + \frac{1}{3} \mathcal{P} g_F m_F \frac{\delta_{\text{FS}}}{\delta} \right) I(\mathbf{r}) \quad (33)$$

where  $c$  is the speed of light,  $\Gamma$  is the atomic linewidth,  $\mathcal{P}$  is the polarization of the light,  $g_F$  is the  $g$ -factor of the hyperfine sublevels,  $m_F$  is the total angular momentum projection quantum number, and  $\delta_{\text{FS}}$  is the fine-structure splitting of the atoms; the polarization dependent term results from the vector light shift (VLS)[8]. We change the polarization  $\mathcal{P} \in [-1, 1]$  of the infrared light propagating along the  $z$ -axis using a  $\lambda/4$ -plate; the resulting VLS modifies the trap depth by  $\mathcal{P} \cdot 20$  nK (a change of up to 0.03%) and the trap frequency along  $x$  by  $\mathcal{P} \cdot 0.06$  Hz (a change of up to 0.015%). However, this leads to a predicted change in the effective curvature along  $x, y$  by  $\mathcal{P} \cdot 200$  G/cm<sup>2</sup>, about 3 times greater than the observed curvature change. The resulting variations in inhomogeneity  $\tilde{h}$  allow us to explore vertically in the dynamical phase diagram of Fig. 2.

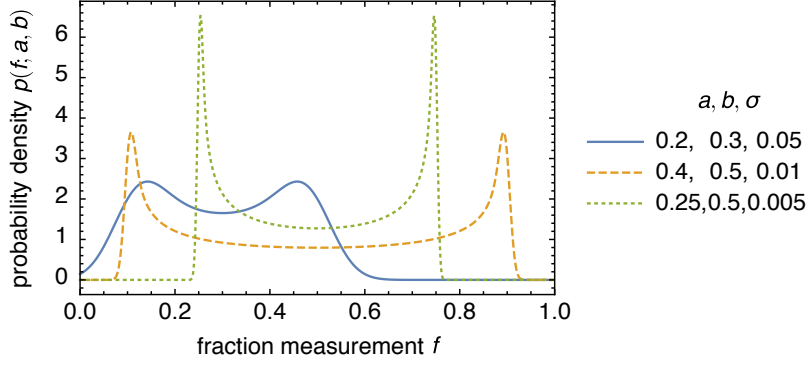

FIG. 5. Probability densities  $p(f; a, b)$  with Gaussian measurement noise width  $\sigma$  for different values of  $a, b, \sigma$  (shown in the legend). From many experimental runs, we determined  $\sigma = 0.01$  for our experimental conditions.

### B. Measurement

To measure magnetization dynamics, we begin by applying an rf pulse resonant with the  $|\uparrow\rangle$  to  $|\downarrow\rangle$  transition which transfers each spin to a coherent superposition  $|\psi\rangle = \frac{1}{\sqrt{2}}(-i|\uparrow\rangle + |\downarrow\rangle)$  at  $t = 0$ , giving collective spin  $S_0^X = 0, S_0^Y = N/2$  (a  $\pi/2$ -pulse). After an interaction time  $t$ , we apply a second  $\pi/2$ -pulse with phase offset  $\theta$  from the initial  $\pi/2$ -pulse to project  $S^X, S^Y$  back into the  $|\uparrow\rangle, |\downarrow\rangle$  populations:  $N_{\uparrow(\downarrow)} = N/2 \pm (S^Y \cos \theta + S^X \sin \theta)$ . Each experimental image measures  $N_{\uparrow}, N_{\downarrow}$ , from which we compute a fraction of  $|\uparrow\rangle$ :

$$\begin{aligned} f &= \frac{N_{\uparrow}}{N_{\downarrow} + N_{\uparrow}} \\ &= \frac{1}{2} + \frac{S^Y}{N} \cos \theta + \frac{S^X}{N} \sin \theta. \end{aligned} \quad (34)$$

The collective spin has projections  $S^Y = S \cos \phi, S^X = S \sin \phi$ , where  $\phi$  is the atomic phase accumulated during  $t$ . We are sensitive to the relative frequency between the drive and the atomic frequency with a precision of  $\sim 1/t$ . For  $t \geq 1.5$  ms we find that our shot-to-shot field stability is insufficient to produce a reproducible phase [9]. This yields  $f = \frac{1}{2} + \frac{S}{N} \cos(\theta')$ , where  $\theta' = \theta - \phi$  is a random phase. To reconstruct the offset  $b$  and amplitude  $a$  of a Ramsey fringe  $F = b + a \cos(\theta')$  from a set of fractions  $f_i$  acquired in several experimental runs with the same conditions, we assume a probability distribution

$$p(f; a, b) = \frac{1}{\sqrt{2\pi}\sigma\pi} \int_0^\pi d\theta' \exp\left(\frac{-(a \cos \theta' + b - f)^2}{2\sigma^2}\right), \quad (35)$$

which is a convolution of the noise-free probability distribution and Gaussian noise with width  $\sigma$ . From many experimental runs, we determine  $\sigma = 0.01$ . Some example distributions are shown in Fig. 5. We construct a log-likelihood function for a set of  $n$  fraction measurements,

$$\ell(a, b; \{f_i\}) = \frac{1}{n} \sum_{i=1}^n \log(p(f_i; a, b)), \quad (36)$$

from which we numerically compute the maximum likelihood estimator (MLE) for the amplitude  $a$  and offset  $b$ , as well as confidence intervals. Where the MLE offset parameter  $b$  falls outside the range  $0.50 \pm 0.05$ , we discard the data, otherwise, the peak-to-peak amplitude  $2a$  gives an estimate for the magnetization  $2S/N$ .

### C. Determining the zero-crossing of the $^{40}\text{K}$ Feshbach resonance

Using a Ramsey sequence, we measure the magnetization  $2S/N$  remaining after  $t = 100$  ms for various bias fields. We fit the resulting magnetization near the zero crossing in the range 208.5–209.5 G for several such data sets with different initial  $N, T$ , acquired over several months, to a Gaussian with constant offset (see Fig. 6A–C). Combining

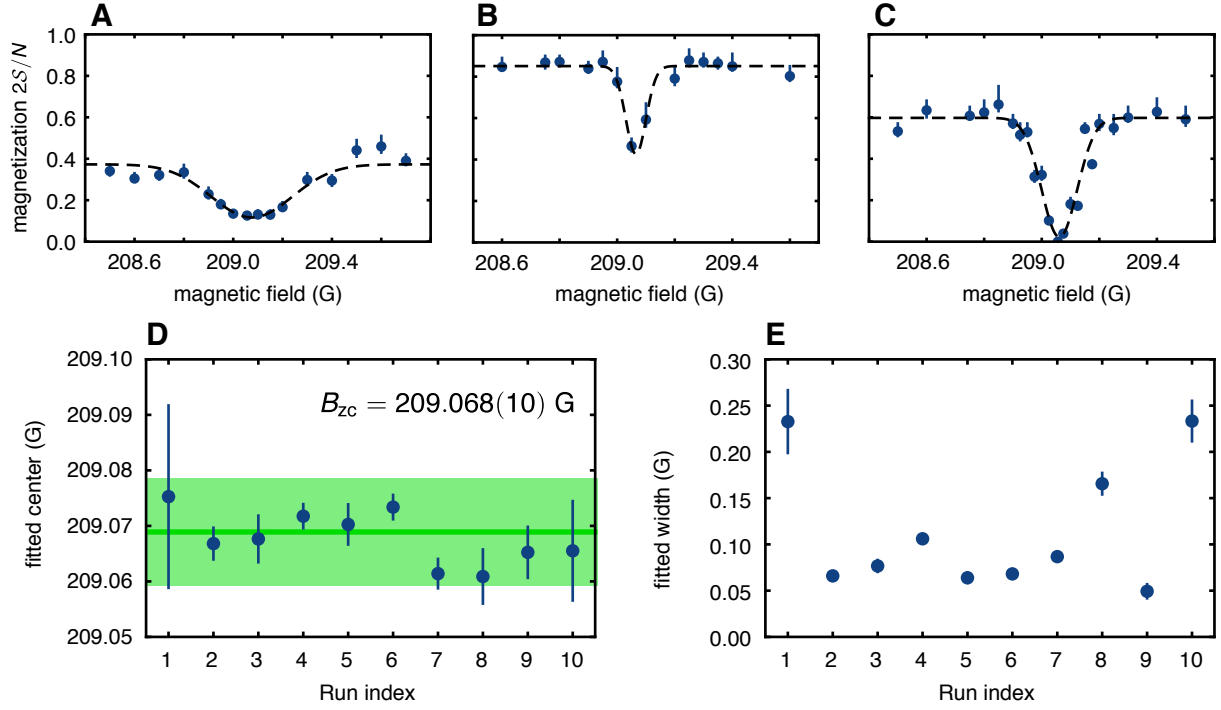

FIG. 6. (A,B,C) Magnetization as a function of magnetic field after 100 ms hold time. Shown are runs taken across six months, with slightly different trap alignments, atom numbers, and temperatures. (D) Best-fit centers from ten data runs. The statistical uncertainty is 5 mG, but we show a systematic uncertainty of 10 mG from typical field drift during a data run. (E) Best-fit Gaussian widths.

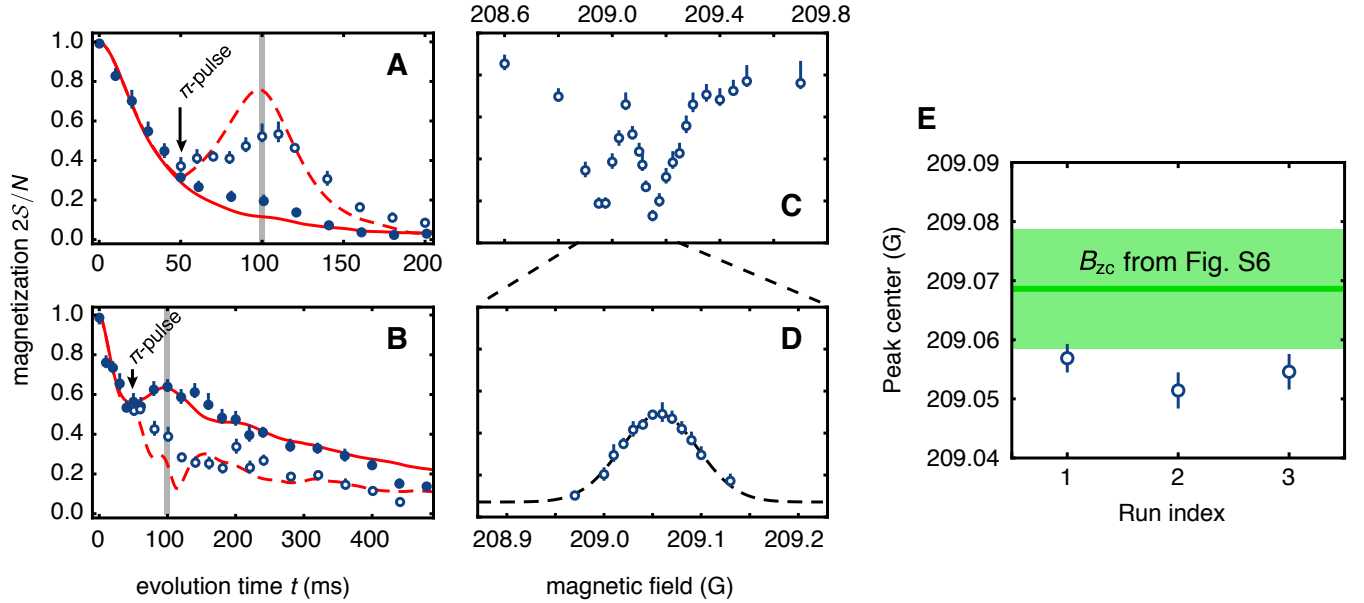

FIG. 7. Magnetization as a function of time with (open points) and without (solid points) a spin-reversal  $\pi$ -pulse at 50 ms (A) for  $B = 209.056(10)$  G,  $N = 2.7(1) \times 10^4$ , and  $k_B T = 0.33(2)E_F$ , and (B) for  $B = 209.175(10)$  G,  $N = 2.9(1) \times 10^4$ , and  $k_B T = 0.30(2)E_F$ . Theory curves are for  $a = -0.5a_0$  and  $a = 2.4a_0$ , respectively. (C) Magnetization versus magnetic field at a fixed total hold time of 100 ms (grey bars in A and B), after a  $\pi$ -pulse at 50 ms. The magnetization shows a characteristic 'W' shape. (D) Denser scan in field to determine center of the 'W'. (E) Best-fit centers, shown with statistical uncertainty only, fall outside the expectation from fits of 'U' profiles (see Fig. 6).

these fit parameters, we find the zero-crossing field  $B_{zc} = 209.068(10)$  G, where the uncertainty is dominated by systematic uncertainty in our bias field (as described in IV).

We compare this result to previous experimental results in Table I. In some cases, the location and width of the Feshbach resonance [10] were measured, so  $B_{zc}$  is only inferred. In the vicinity of  $B_{zc}$ , the  $s$ -wave scattering length  $a$  varies linearly in magnetic field with slope  $a_{bg}/\Delta$ , where  $a_{bg} = 169.67(24) a_0$  [11] and  $a_0 \approx 0.0529$  nm is the Bohr radius. Our measurement improves the uncertainty of  $B_{zc}$  by an order of magnitude. Although we have not determined the resonance field  $B_0$  independently in this work, if our  $B_{zc}$  is combined with  $B_0 = 202.10(7)$  G [12], then the width of the resonance is  $\Delta = 6.97(8)$  G. Scattering lengths in this work are calculated from measured magnetic fields using  $B_{zc} = 209.07(1)$  G,  $B_0 = 202.10(7)$  G, and  $a_{bg} = 169.67(24) a_0$ .

| $B_0$ (G)         | $\Delta$ (G)    | $B_{zc}$ (G)     | $a_{bg}(a_0)$ | Method                           |                      |
|-------------------|-----------------|------------------|---------------|----------------------------------|----------------------|
| <b>201.5(1.4)</b> | <b>8.0(1.1)</b> | 209.5            | 174           | cross-dimensional thermalization | Jin [13]             |
| <b>202.10(7)</b>  | 8               | 209.1            | 174           | molecular dissociation           | Jin [12]             |
| <b>202.20(2)</b>  | <b>7.1(2)</b>   | 209.3            | 174           | molecule rf spectroscopy         | Jin [14]             |
| 202.1             | 7.5             | <b>209.6(1)</b>  | 174           | dephasing of Bloch oscillations  | Esslinger [15] p. 65 |
| 202.1             | 7.0             | <b>209.1(2)</b>  | 174           | lattice expansion dynamics       | Bloch [16]           |
| <b>202.14(1)</b>  | <b>6.70(3)</b>  | 208.84           | 169.7         | molecule rf spectroscopy         | Sagi [17]            |
| 202.1             | 6.97            | <b>209.07(1)</b> | 169.67        | many-body magnetization dynamics | this work            |

TABLE I. Comparison of experimental determinations of the  $s$ -wave Feshbach zero-crossing field  $B_{zc}$ , the Feshbach resonance location  $B_0$  and width  $\Delta$ , as well as the background scattering length  $a_{bg}$  used to parameterize the resonance. Directly measured quantities are indicated in boldface, while inferred or assumed values are in regular font.

An alternate procedure to determine the zero-crossing is to look for a local peak in spin-echo magnetization. If we apply a spin-reversal rf pulse, or  $\pi$ -pulse, at  $t = 50$  ms, the subsequent evolution of the magnetization depends strongly on the scattering length  $a$ . Near  $a = 0$ , the spin reversal leads to nearly full recovery of the magnetization, as seen in Fig. 7A. Near the onset of gap protection, however, near  $|a| \approx 3a_0$ , the spin echo induced by the reversal pulse competes with the spin self-rephasing and leads to decreased magnetization [18], as seen in Fig. 7B. At a fixed interaction time of  $t = 100$  ms with spin reversal at  $t = 50$  ms, we vary the field near  $a = 0$  and observe the magnetization follows a ‘W’ shape (see Fig. 7C). We measure the central lobe of the ‘W’ shape a few times over several months with slightly different trap alignments and initial  $N, T$  and fit the central lobes to Gaussian profiles with constant offset to find the center locations; one such fit is shown in Fig. 7D. The resulting center fields are significantly lower than  $B_{zc}$  found without spin reversal, represented as the band in Fig. 7E. A possible cause is the presence of the constant magnetic field gradient  $\Delta\mathcal{B}$ . As shown in Fig. 4, in the vicinity zero-crossing field, with the addition of a spin echo pulse, the amplitude of the fast oscillation induced by the constant gradient is non-negligible and might cause the shift of  $B_{zc}$ .

## V. DATA ANALYSIS FOR FINE EXPLORATION OF DPT (FIGURE 3)

This section describes the data analysis for Fig. 3 in the main text, exploring the change in dynamics across the DPT. Roughly 7000 cycles of the experiment were used to create a data set of  $\mathcal{S}$  versus hold time at  $\tilde{h} = 2\pi \times 18(1)$  Hz. This value of  $\tilde{h}$  is realized with a fully circular polarization of the trapping beam (as in Fig. 2B), atom number  $N = 3.0 \times 10^4$ , and temperature  $T = 0.5T_F$  (higher than the data for Fig. 2). We discard any measurements of  $\mathcal{S}$  with mean fraction outside  $0.50 \pm 0.05$ , and any initial measurements that are anomalously low. Furthermore, time sampling was restricted to multiples of 2.5 ms, the trap period, to lessen the effect of single-particle oscillations (see Sec. III) especially at short hold times. These cuts left 6300 simulation runs, across 21 time series, which we compared systematically to numerical calculations. Model calculations were scaled with a phenomenological factor of  $\exp(-\Gamma_0 t)$ , where  $\Gamma_0 = 1.75 \text{ s}^{-1}$ , as described in the main text and used in Figs. 2 and 4. The correction for collisions was not used here ( $\gamma \rightarrow 0$ ).

The first analysis step compares the time series to the mean-field calculation of non-interacting dynamics (i.e.,  $a = 0$ ), which we label  $S_{J=0}(t)$ . Interacting data is fit to  $S_{J=0}(\kappa t)$ , with  $\kappa$  as the sole fit parameter. The  $\chi^2$  of this fit identifies the qualitative departure from non-interacting dynamics as a step in  $\chi^2$ . The result is shown in Fig. 3F. Uncertainties on the  $\chi^2$  for each time series are determined by Monte Carlo sampling each data set. For each time series we create  $10^4$  new data sets by sampling the original time series with replacement. Each data set has the same number of points as the time series it is sampled from. Fitting this ensemble of data sets produces a roughly Gaussian distribution of  $\chi^2$ . The mean and standard deviation are shown in Fig. 3F as the center value and the uncertainty.

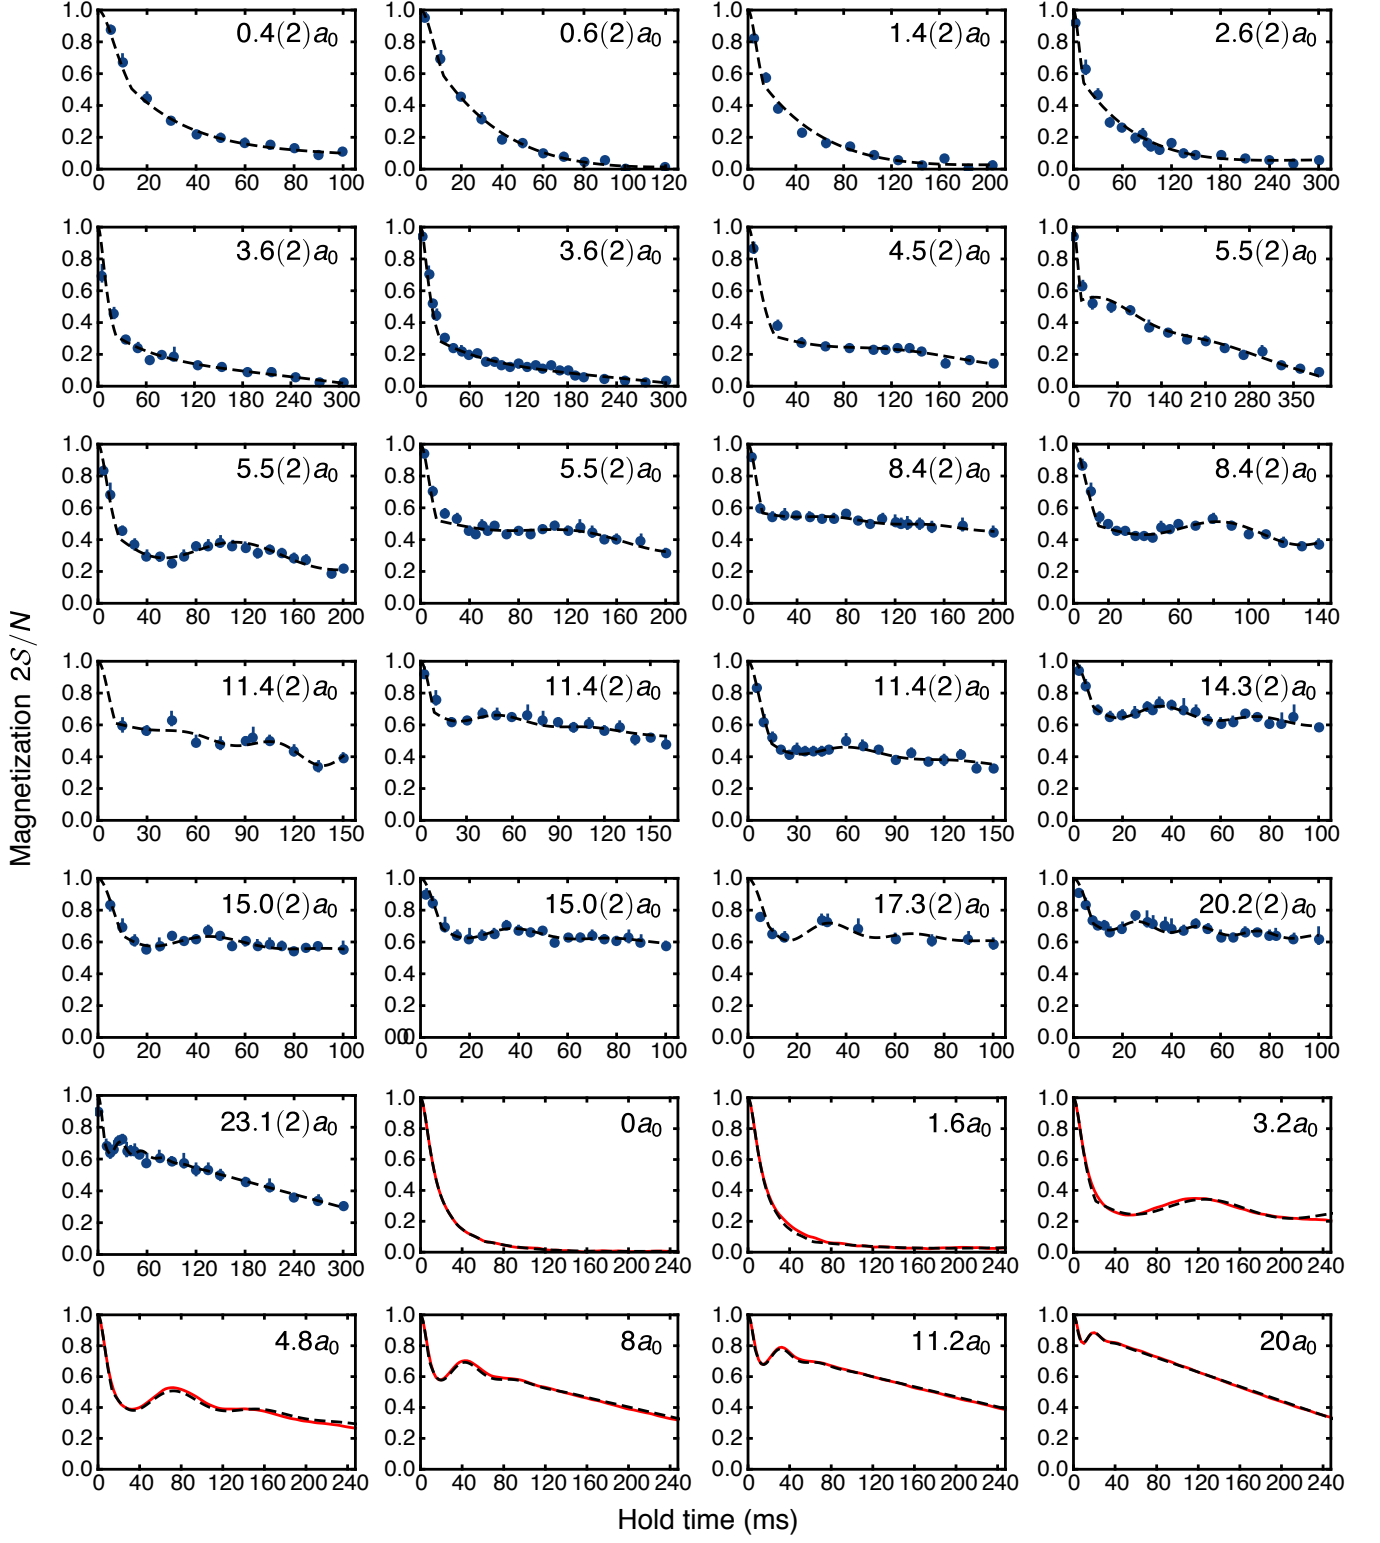

FIG. 8. **Fits to time series.** Magnetization as a function of time for different scattering lengths. Blue points are experimental data with error bars reflecting statistical uncertainty; red lines are numerical theory; dashed lines are fits to the function Eq. 37, as described in Sec. V. The conditions of the data and theory are those for Fig. 3 in the main text.

This analysis gives a first indication of the phase transition: data above the critical scattering length  $a_c \sim 3a_0$  have a significantly increased  $\chi^2$ .

To extract a frequency from our data, we fit data to the function

$$S_{\text{fit}}(t) = \begin{cases} S_{J=0}(t) & \text{for } t \leq t_G \\ S_{J=0}(t_G) + m_s(t - t_G) + Ae^{-\xi t} \cos(\Omega(t - t_G)) & \text{for } t > t_G \end{cases} \quad (37)$$

with four fit parameters:  $t_G$  (“gap time”), frequency  $\Omega$ , spin-wave damping rate  $\xi$ , and slope  $m_s$ . The form of  $S_{\text{fit}}(t)$  relies on the universality of early-time dynamics (depending only on  $\tilde{h}$ ), and the ansatz of gapped dynamics with fixed  $\Omega$  at later times. The fitting procedure is iterative: a first round uses  $A = 0$ , to determine  $m_s$ ; a second pass holds  $m_s$  fixed and varies the remaining four parameters. Fits are seeded with initial conditions that select a local minimum, so that analysis uncertainties are insensitive to the full complexity of optimization. All fits to data and some examples of fits to theory are shown in Fig. 8.

As expected in the demagnetized phase, fits to extract a frequency are poor for data taken at scattering lengths of less than  $\sim 4a_0$ . Above the transition,  $\chi^2$  per degree of freedom in fits to Eq. 37 is typically  $\simeq 2$ . From the fits we extract the frequencies  $\Omega$ , which we use as an order parameter and which we show in Fig. 3H. From the same  $S_{\text{fit}}(t)$  with best-fit parameters, we interpolate a value for  $\mathcal{S}$  at  $t = 100$  ms, as a function of scattering length, as another signature of the DPT. The results are shown in Fig. 3G in the main text.

To determine the location of the DPT, we fit the order parameter with the form

$$\Omega(NJ) = \frac{\pi}{2} \beta NJ_c \cot\left(\frac{NJ_c \pi}{NJ} \frac{\pi}{2}\right) \quad (38)$$

where  $NJ_c$  is the critical interaction strength and  $\beta$  is a scaling factor. Compared with Eqn. 22, we find  $NJ_c = 2\sqrt{3}\alpha\tilde{h}/(\beta\pi)$ . We combine our knowledge of the step in  $\chi^2$ , and the poor fit confidence to exclude frequencies from time series below  $3a_0$ . The frequencies excluded are shown in grey in Fig. 3H in the main text. Despite the fact that this functional form is only strictly correct in the 1D all-to-all model (Sec. 4), we find that the frequency in the gapped phase is still linear in  $J$ , but with a scaling factor  $\beta$  that reflects the reduction of collectivity due to the reduction of  $\mathcal{J}_{ij}$  with mode distance (see Sec. IB). The best-fit location of the dynamical critical point is  $NJ_c/2\pi = 7.8(1.1)$  Hz, or a critical scattering length  $a_c = 2.8(4)a_0$ , with a scaling factor  $\beta = 0.56(1)$ . This implies renormalization factors  $\alpha = \beta\pi NJ_c/2\sqrt{3}\tilde{h} \simeq 0.22(3)$  and  $\beta \simeq 0.56(1)$ .

Figures 3G,H also show this same analysis procedure applied to the theoretical mean-field numerical results (Sec. 3). All the same signatures of the DPT are observed. However, this agreement includes an overall scaling of the  $\mathcal{J}_{ij}$  by 0.8 from their ab-initio values. As discussed in the main text, this is perhaps due to an increased sampling of trap anharmonicity due to the higher temperature used in this data set to increase  $\tilde{h}$ , or due to a renormalization of coupling constants due to resonant mode-changing processes [7, 19]. For the non-thermally averaged data (solid black lines in Fig. 3), we find  $NJ_c/2\pi = 4.98(0.14)$  Hz, or a critical scattering length  $a_c = 1.78(5)a_0$ , with a scaling factor  $\beta = 0.55(2)$ . For the thermally averaged data (red lines in Fig. 3), we find  $NJ_c/2\pi = 3.75(0.25)$  Hz, or a critical scattering length  $a_c = 1.34(9)a_0$ , with a scaling factor  $\beta = 0.54(2)$ . The difference of the best-fit location of the DPT between the two theoretical data is due to the fact that thermal averaging washes out the oscillation and induces global dephasing that reduces the contrast. This reflects a high sensitivity to dephasing and parameter drift near the critical point, in experimental runs. Furthermore, the finite time window of measurement and simulation limits the accuracy of  $\Omega$  near the critical point, where the period of oscillation diverges.

## VI. SCATTERING RATE OF THE NON-EQUILIBRIUM GAS

In this section, we estimate the collision rate using a kinetic theory. The semi-classical distribution function  $f(\mathbf{x}, \mathbf{p}, t)$  (normalized to  $(2\pi\hbar)^{-3} \int d^3\mathbf{x} d^3\mathbf{p} f = N$ ) is changed due to collisions at a rate

$$C[f(\mathbf{x}, \mathbf{p}_1, t)] = \iint \frac{d^3\mathbf{p}_2}{(2\pi\hbar)^3} \frac{d^3\mathbf{p}_3}{(2\pi\hbar)^3} W(\mathbf{x}, \mathbf{p}_1, \mathbf{p}_2, \mathbf{p}_3, \mathbf{p}_4) \delta(\epsilon_1 + \epsilon_2 - \epsilon_3 - \epsilon_4) \times \{f_1 f_2 (1 - f_3)(1 - f_4) - f_3 f_4 (1 - f_1)(1 - f_2)\} \quad (39)$$

where  $f_1 = f(\mathbf{x}, \mathbf{p}_1, t)$ , etc.;  $W(\dots)$  is the scattering probability from 1, 2 to 3, 4; and  $\mathbf{p}_4$  is fixed by conservation of momentum. In equilibrium,  $C[f_{\text{eq}}] = 0$ , because the scattering rate into each volume in phase space is equal to the

scattering rate out. We can separate these two rates, as  $C(\mathbf{x}, \mathbf{p}) = C^+ - C^-$ , and define the total collision rate as

$$\dot{N}_{\text{coll}} = \iint \frac{d^3\mathbf{x} d^3\mathbf{p}_1}{(2\pi\hbar)^3} C^+(\mathbf{x}, \mathbf{p}_1). \quad (40)$$

With local translational symmetry and  $s$ -wave interactions,

$$C^+[f(\mathbf{x}, \mathbf{p}_1)] = \int \frac{d^3\mathbf{p}_2}{(2\pi\hbar)^3} \int d\Omega \frac{d\sigma}{d\Omega} |\mathbf{v}_1 - \mathbf{v}_2| f_1 f_2 (1 - f_3)(1 - f_4) \quad (41)$$

where  $f_1 = f(\mathbf{x}, \mathbf{p}_1)$ , etc [20]. In the low-energy, momentum-independent limit,  $d\sigma/d\Omega = \sigma/4\pi$ ,  $\sigma = 4\pi a^2$ . In this case,

$$\dot{N}_{\text{coll}} = \sigma \iiint d^3\mathbf{x} \frac{d^3\mathbf{p}_1}{(2\pi\hbar)^3} \frac{d^3\mathbf{p}_2}{(2\pi\hbar)^3} \frac{d\Omega}{4\pi} |\mathbf{v}_1 - \mathbf{v}_2| f_1 f_2 (1 - f_3)(1 - f_4) \quad (42)$$

where  $d\Omega = d\phi \cos\theta d\theta$ , and  $\phi, \theta$  give the angles of  $\mathbf{p}_3 - \mathbf{p}_4$ .

### A. Equilibrium scattering rate

For a degenerate Fermi gas in an equal mixture of two spin states, Lepers *et al.* [20] write

$$\dot{N}_{\text{coll,FG}} = \frac{1}{4\pi^4} \int d^3\mathbf{r} \int_0^\infty dk k^2 \int_0^\infty dq q^2 \frac{2q}{m} \sigma(q) \left[ \frac{\tanh^{-1}(\tanh \frac{X}{2} \tanh \frac{Y}{2})}{Y \sinh X} \right]^2 \quad (43)$$

where  $X \equiv \beta(k^2/8m + q^2/2m + V_T - \mu)$  and  $Y \equiv \beta kq/2m$ . For a harmonic trap  $V_T$ , we can rescale the spatial coordinates to be spherically symmetric, and then pull all dimensional factors out of the integral for  $r, k$ , and  $q$ . Using  $V_T = \frac{1}{2}m\omega^2 r^2 \rightarrow r'^2/2$ ,  $\beta k^2/m \rightarrow k'^2$ , the integrations are  $d^3\mathbf{r} = (\beta m\omega^2)^{-3/2} 4\pi r'^2 dr'$  and  $dk k^2 = (m/\beta)^{3/2} dk' k'^2$ . Now (dropping primes)  $X \rightarrow k^2/8 + q^2/2 + r^2/2 - \mu\beta$  and  $Y \rightarrow kq/2$ , such that

$$\dot{N}_{\text{coll,FG}} = \frac{2}{\pi^3} \frac{m\sigma}{\beta^5 \omega^3} \underbrace{\int_0^\infty dr r^2 \int_0^\infty dk k^2 \int_0^\infty dq q^3 \left[ \frac{\tanh^{-1}(\tanh \frac{X}{2} \tanh \frac{Y}{2})}{Y \sinh X} \right]^2}_{\equiv F(\beta\mu)}.$$

Using the relation  $N_\uparrow(\beta\omega)^3 = -\text{Li}_3(-z_\uparrow)$ , where  $\text{Li}_3$  is a polylog function and  $z = e^{\beta\mu}$  is the fugacity, we insert two factors of number:

$$\frac{\dot{N}_{\text{coll,FG}}}{N_\downarrow} = \left( \frac{N_\uparrow}{2\pi^2} m\sigma\beta\omega^3 \right) \frac{4F(\beta\mu)}{\pi \text{Li}_3(-z_\uparrow) \text{Li}_3(-z_\downarrow)} \quad (44)$$

In this form, the collision rate of the Fermi gas can be compared to the collision rate of a spin mixture in the Maxwell-Boltzmann limit,

$$\frac{\dot{N}_{\text{coll,Boltz}}}{N_\downarrow} \rightarrow \frac{1}{2\pi^2} N_\uparrow m\sigma\beta\omega^3 \quad (45)$$

The two effects of Fermi degeneracy are a change in position and momentum distributions, and the blocking of collisions due to occupied final states. Lepers *et al.* provide a formula that neglects the latter: the rate of all collisions (even those that are blocked) is [20]

$$\dot{N}_{\text{coll,FG}}^{(+\text{blocked})} = \frac{1}{4\pi^4} \int d^3\mathbf{r} \int_0^\infty dk k^2 \int_0^\infty dq q^2 \frac{2q}{m} \sigma(q) \frac{\tanh^{-1}(\tanh \frac{X}{2} \tanh \frac{Y}{2})}{Y e^X \sinh X} \quad (46)$$

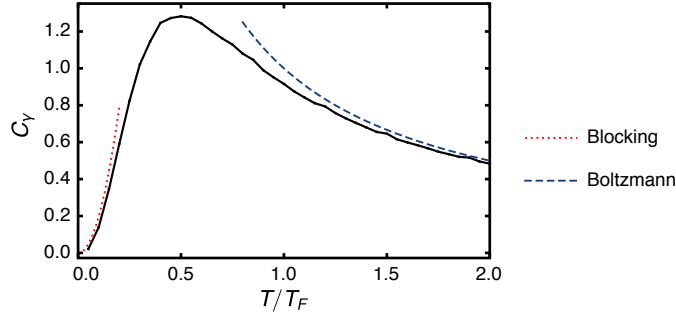

FIG. 9. **Dimensionless collision rate versus temperature.** This is a plot of Eq. 51. The coefficient is chosen to be  $\beta E_F$  at high temperature (blue dashed line). The low-temperature behavior is dominated by blocking (dotted red line). From this dimensionless  $C_\gamma$ , one finds the scattering rate by multiplying by  $\gamma_0 = N_\uparrow m \sigma \omega^3 / 2\pi^2 E_F$ .

which results in an expression like Eq. 44, but with

$$F^{(+\text{blocked})}(\beta\mu) = \int_0^\infty dr r^2 \int_0^\infty dk k^2 \int_0^\infty dq q^3 \frac{\tanh^{-1}(\tanh \frac{X}{2} \tanh \frac{Y}{2})}{Y e^X \sinh X} \quad (47)$$

The low-temperature limit of Eq. 46 is

$$\frac{\dot{N}_{\text{coll}}^{(+\text{blocked})}}{N_\downarrow} \approx 0.21 \frac{N_\uparrow m \sigma \omega^3}{E_F} \quad (48)$$

which scales as one would expect from  $n\sigma v_{\text{rel}}$ , with a Thomas-Fermi cloud shape and an average relative velocity proportional to the Fermi velocity.

Blocking will further reduce the collision rate as  $(T/T_F)^2$  at low temperature. This can be calculated by taking the ratio of the two dimensionless integrals:

$$r_{\text{allowed}} \equiv \frac{\dot{N}_{\text{coll}}}{\dot{N}_{\text{coll}}^{(+\text{blocked})}} = \frac{F(\beta\mu)}{F^{(+\text{blocked})}(\beta\mu)} \rightarrow \text{const.} \times \frac{T^2}{E_F^2} \quad (49)$$

At low temperature, “const.” is  $\approx 5$ , so that

$$\frac{\dot{N}_{\text{coll}}}{N_\downarrow} \approx 1.0 \frac{N_\uparrow m \sigma \omega^3}{E_F} \frac{T^2}{E_F^2} \quad \text{for } T \ll T_F \quad (50)$$

This is roughly equal to (but slightly higher than) the value given by O’Hara *et al.* [21], who give a pre-factor of  $15/2\pi^2 \approx 0.76$  at low temperature.

Figure 9 summarizes these results in dimensionless form: the scattering rate is

$$\frac{\dot{N}_{\text{coll}}}{N_\downarrow} = C_\gamma \gamma_0 \quad \text{where} \quad \gamma_0 \equiv \frac{N_\uparrow m \sigma \omega^3}{2\pi^2 E_F} \quad \text{and} \quad C_\gamma = \frac{4\beta E_F F(\beta\mu)}{\pi \text{Li}_3(-z_\uparrow) \text{Li}_3(-z_\downarrow)} \rightarrow \begin{cases} (T/T_F)^{-1} & \text{for } T \gg T_F, \\ 2\pi^2 (T/T_F)^2 & \text{for } T \ll T_F \end{cases} \quad (51)$$

with a peak value  $C_\gamma \approx 1.3$  at  $T \approx 0.5 T_F$ , in agreement with Ref. [21].

For our typical experimental parameters, with  $2N_\uparrow = 3 \times 10^4$   $^{40}\text{K}$  atoms in a trap with  $\omega/2\pi = \{393, 1140, 950\}$  Hz, the reference scattering rate is  $\gamma_0 = 0.0084 \text{ s}^{-1} (a/a_0)^2$  where  $a_0$  is the Bohr length. For  $0.5 T_F$ , we multiply by  $C_\gamma = 1.3$  (see Fig. 9) to find a scattering rate of  $0.011 \text{ s}^{-1}$  times  $(a/a_0)^2$ .

## B. Finite polarization, prepared out of equilibrium

This calculation so far has considered an unpolarized mixture, characterized by a single chemical potential, and an equal number of particles. For an imbalanced non-degenerate mixture, Eq. 45 tells us that  $\dot{N}_{\text{coll}} \propto N_\uparrow N_\downarrow$ . The collision rate per particle depends on which type of particle interests us:  $\dot{N}_{\text{coll}}/N_\uparrow \propto N_\downarrow$ , and  $\dot{N}_{\text{coll}}/N_\downarrow \propto N_\uparrow$ . In

other words, the scattering rate of the majority species is highly sensitive to polarization, but scattering rate seen by impurities is relatively insensitive. Choosing  $N_\uparrow$  to be the majority population, we can define both polarization  $P$  and a minority fraction  $x$ , such that

$$N_\uparrow/N = (1 + P)/2 = (1 - x) \quad (\text{majority}) \quad \text{and} \quad N_\downarrow/N = (1 - P)/2 = x \quad (\text{minority}) \quad (52)$$

Or, written in comparison to an unpolarized gas,  $N_{\uparrow,\downarrow} = (N/2)(1 \pm P)$ . Then the scattering rates scale as

$$\frac{\dot{N}_{\text{coll,Boltz}}}{N_{\uparrow,\downarrow}} = N_{\downarrow,\uparrow} \frac{m\sigma\beta\omega^3}{2\pi^2} = \left( \frac{\dot{N}_{\text{coll,Boltz}}}{N/2} \right)_{P=0} \times (1 \mp P) \quad (\text{trapped Boltzmann gas}) \quad (53)$$

In other words, the total (extensive) collision rate scales as  $1 - P^2$ , or  $4x(1 - x)$ , for constant  $\beta$ .

An estimate of the polarization in our experiment comes from the maximum contrast in a Ramsey sequence. The visibility of a fringe is  $\mathcal{V} = (N_{\text{max}} - N_{\text{min}})/(N_{\text{max}} + N_{\text{min}})$ . For a mixture with  $N_\uparrow > N_\downarrow$ , this visibility is

$$\mathcal{V} = \frac{N_\uparrow - N_\downarrow}{N} = 1/2 + P/2 - (1/2 - P/2) = P \quad (54)$$

So, the upper bound of fringe visibility is  $P$ . For our best data sets, this is  $P \approx 0.8$ , such that the scattering rate per majority particle is  $\approx 0.2$  times the rate that would be estimated for a balanced thermal gas.

For a degenerate gas, we need to be more careful when applying this correction. An imbalanced gas would have different spatial distributions, momentum distributions, and blocking factors for the minority and majority populations.

In our experiment, the gas is initialized when fully polarized (but at finite temperature). We assume that some de-polarization occurs, but without rearrangement among non-interacting eigenstates. We furthermore assume that the depolarization is uniform among all occupied states. Calling the majority  $\downarrow$ , the occupation functions for the two spin states can then be written

$$f_\uparrow = (N_\uparrow/N)f^i \equiv xf^i \quad \text{and} \quad f_\downarrow = (N_\downarrow/N)f^i = (1 - x)f^i \quad (55)$$

where  $f^i$  is the distribution of the initially polarized gas.

These distribution functions are then put into the scattering rate Eq. 40,

$$\begin{aligned} \dot{N}_{\text{coll,pol}} &= \int \frac{d^3\mathbf{x} d^3\mathbf{p}_1}{(2\pi\hbar)^3} C^+(\mathbf{x}, \mathbf{p}_1) \\ &= \iiint \frac{d^3\mathbf{x} d^3\mathbf{p}_1}{(2\pi\hbar)^3} \frac{d^3\mathbf{p}_2}{(2\pi\hbar)^3} \frac{d^3\mathbf{p}_3}{(2\pi\hbar)^3} W_{1234} \delta(\Delta\epsilon) f_{\downarrow,1} f_{\uparrow,2} (1 - f_{\downarrow,3}) (1 - f_{\uparrow,4}) \\ &\equiv \langle f_{\downarrow,1} f_{\uparrow,2} \rangle - \langle f_{\downarrow,1} f_{\uparrow,2} f_{\downarrow,3} \rangle - \langle f_{\downarrow,1} f_{\uparrow,2} f_{\uparrow,4} \rangle + \langle f_{\downarrow,1} f_{\uparrow,2} f_{\downarrow,3} f_{\uparrow,4} \rangle \\ &= x(1 - x) \langle f_1^i f_2^i \rangle - x(1 - x) \langle f_1^i f_2^i f_3^i \rangle + x^2(1 - x) \langle f_1^i f_2^i f_3^i f_4^i \rangle \end{aligned} \quad (56)$$

where in the last line we have used  $\langle f_1^i f_2^i f_3^i \rangle = \langle f_1^i f_2^i f_4^i \rangle$ .

We can relate many of these  $\langle \dots \rangle$  terms to equilibrium scattering rates, because  $f^i$  is the distribution of a single spin state in an *equilibrium* Fermi gas, which is also the distribution of either spin state in a balanced Fermi gas with  $2N$  atoms, but the same  $T/T_F$ . For instance, taking only the first term,

$$\dot{N}_{\text{coll,pol}} = x(1 - x) \langle f_1^i f_2^i \rangle = x(1 - x) \dot{N}_{\text{coll,FG}}^{(+\text{blocked})} \Big|_{\text{unpol}, 2N} \quad (57)$$

which is calculated using Eq. 46. To see that this is correct in the high temperature limit, we use Eq. 45:

$$\dot{N}_{\text{coll,FG}}^{(+\text{blocked})} \Big|_{\text{unpol}, 2N} \rightarrow N^2 \frac{m\sigma\beta\omega^3}{2\pi^2} \quad \text{so that} \quad \dot{N}_{\text{coll,pol}} \rightarrow N_\uparrow N_\downarrow \frac{m\sigma\beta\omega^3}{2\pi^2} \quad (58)$$

since  $x(1 - x)N^2 = N_\uparrow N_\downarrow$ . This agrees with Eq. 53. However, the full expression, Eq. 57, correctly includes the FD modification of the initial distribution.

Next, we find an estimate of Pauli blocking in the weakly degenerate regime. This relies upon the assumption that

$$x(1 - x) \langle f_1^i f_2^i f_3^i f_4^i \rangle \ll \langle f_1^i f_2^i f_4^i \rangle \quad (59)$$

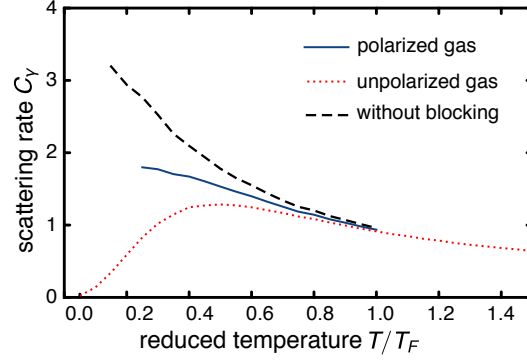

FIG. 10. **Dimensionless collision rate of majority population.** The dimensionless collision rate per spin- $\downarrow$  atom is plotted versus temperature. The “polarized gas” estimate (solid blue line) is from Eq. 61; it exceeds the normalized equilibrium rate (dotted red line) for an unpolarized gas because Pauli blocking is absent for the final states of a minority population in the strong-polarization limit  $x \ll 1$  (see text).

which would be an appropriate assumption if  $x \ll 1$  and/or  $f \ll 1$ . In the equilibrium balanced gas of  $2N$  particles,

$$r_{\text{allowed}} = \frac{\langle f_1 f_2 - 2f_1 f_2 f_3 + f_1 f_2 f_3 f_4 \rangle}{\langle f_1 f_2 \rangle} \approx 1 + \frac{\langle -2f_1 f_2 f_3 \rangle}{\langle f_1 f_2 \rangle} \quad \text{or} \quad \frac{\langle -f_1 f_2 f_3 \rangle}{\langle f_1 f_2 \rangle} \approx -\frac{1 - r_{\text{allowed}}}{2} \quad (60)$$

and (starting from Eq. 56 and also dropping the four- $f$  term),

$$\begin{aligned} \dot{N}_{\text{coll,pol}} &\approx x(1-x) [\langle f_1^i f_2^i \rangle - \langle f_1^i f_2^i f_3^i \rangle] \\ &\approx x(1-x) \dot{N}_{\text{coll,FG}}^{(+\text{blocked})} \Big|_{\text{unpol},2N} \times \left( 1 - \frac{1 - r_{\text{allowed}}}{2} \right) \end{aligned} \quad (61)$$

In other words, the depolarizing gas of  $N$  particles is “half as blocked” as the equilibrium gas of  $2N$  particles, under the assumption given by Eq. 59. For instance, at  $T = 0.5T_F$ ,  $1 - r_{\text{allowed}} \approx 0.3$ , so for a depolarizing case, the blocking effect is half this, only  $\approx 0.15$ .

With the experimental conditions  $N_{\uparrow} + N_{\downarrow} = 3 \times 10^4$ ,  $\bar{\omega}/2\pi = 750$  Hz, and  $P = 0.8$  or  $x = 0.1$ , these various approximations give the following estimates. Choosing the majority population as a reference, we define the initial Fermi energy  $E_{Fi} = E_F(N_{\downarrow} = N)$ , the initial degeneracy factor  $t_i = k_B T_i / E_{Fi}$ , and the reference scattering rate  $\gamma_0|_{2N} = Nm\sigma\omega^3/2\pi^2 E_{Fi}$ , which for a 3D gas is  $2^{2/3}$  larger than the scattering rate used when discussing an unpolarized gas,  $\gamma_0|_N = (N/2)m\sigma\omega^3/2\pi^2 E_F(N_{\downarrow} = N/2)$ , in the previous section.

At  $k_B T_i = 0.5E_F(N_{\downarrow} = N)$ , the non-degenerate estimate is (from Eq. 53)  $\dot{N}_{\text{coll,Boltz}}/(1-x)N = x\gamma_0|_{2N} t_i^{-1}$  or  $\approx 0.0027 \text{ s}^{-1} (a/a_0)^2$ . For a Fermi gas,  $\dot{N}_{\text{coll,pol}}/(1-x)N$  is  $\approx 0.0020 \text{ s}^{-1} (a/a_0)^2$ , to which blocking contributes 15% reduction.

At  $k_B T_i = 0.3E_F(N_{\downarrow} = N)$ , the non-degenerate estimate is higher ( $0.0044 \text{ s}^{-1} (a/a_0)^2$ ), but now the Fermi distribution makes a 25% effect, the blocking is a 30% effect, and the final rate is comparable:  $0.0024 \text{ s}^{-1} (a/a_0)^2$ . One can see this gentle slope in the “polarized gas” line in Fig. 10.

Since these estimates concur with the best-fit  $\gamma \simeq 0.002 \text{ s}^{-1} (a/a_0)^2$  shown in Fig. 4 in the main text, we conclude that mode-changing collisions are responsible for the  $a$ -dependent breakdown of the spin model. These calculations also predict that an improved polarization (for instance, by further reducing gradients, see Sec. III) and lower temperatures could extend the range of its validity.

- 
- [1] E. A. Yuzbashyan and M. Dzero, Phys. Rev. Lett. **96**, 230404 (2006).
  - [2] E. A. Yuzbashyan, O. Tsyplatyev, and B. L. Altshuler, Phys. Rev. Lett. **96**, 097005 (2006).
  - [3] E. A. Yuzbashyan, M. Dzero, V. Gurarie, and M. S. Foster, Phys. Rev. A **91**, 033628 (2015).
  - [4] A. Gambassi and P. Calabrese, Eur. Phys. Lett. **95**, 66007 (2011).
  - [5] B. Sciolla and G. Biroli, Phys. Rev. B **88**, 201110 (2013).
  - [6] P. Smacchia, M. Knap, E. Demler, and A. Silva, Phys. Rev. B **91**, 205136 (2015).

- [7] A. P. Koller, J. Munding, M. L. Wall, and A. M. Rey, Phys. Rev. A **92**, 033608 (2015).
- [8] R. Grimm, M. Weidemüller, and Y. B. Ovchinnikov, Adv. At. Mol. Opt. Phys. **42**, 95 (2000).
- [9] A. B. Bardson, S. Beattie, C. Luciuk, W. Cairncross, D. Fine, N. S. Cheng, G. J. A. Edge, E. Taylor, S. Zhang, S. Trotzky, and J. H. Thywissen, Science **344**, 722 (2014).
- [10] C. Chin, R. Grimm, P. Julienne, and E. Tiesinga, Rev. Mod. Phys. **82**, 1225 (2010).
- [11] S. Falke, H. Knoeckel, J. Friebe, M. Riedmann, E. Tiemann, and C. Lisdat, Phys. Rev. A **78**, 012503 (2008).
- [12] C. A. Regal, M. Greiner, and D. S. Jin, Phys. Rev. Lett. **92**, 040403 (2004).
- [13] T. Loftus, C. A. Regal, C. Ticknor, J. L. Bohn, and D. S. Jin, Phys. Rev. Lett. **88**, 173201 (2002).
- [14] J. P. Gaebler, J. T. Stewart, T. E. Drake, D. S. Jin, A. Perali, P. Pieri, and G. C. Strinati, Nat. Phys. **6**, 569 (2010).
- [15] J. Jördens, *Metallic and Mott-insulating phases in fermionic quantum gases*, Ph.D. thesis, Thesis, ETH Zürich (2010).
- [16] U. Schneider, L. Hackermüller, J. P. Ronzheimer, S. Will, S. Braun, T. Best, I. Bloch, E. Demler, S. Mandt, D. Rasch, and A. Rosch, Nat Phys **8**, 213 (2012).
- [17] C. Shkedrov, Y. Florshaim, G. Ness, A. Gandman, and Y. Sagi, “High sensitivity rf spectroscopy of a strongly-interacting fermi gas,” arXiv:1803.01770.
- [18] C. Solaro, A. Bonnin, F. Combes, M. Lopez, X. Alauze, J. N. Fuchs, F. Piéchon, and F. Pereira Dos Santos, Phys. Rev. Lett. **117**, 163003 (2016).
- [19] A. P. Koller, M. L. Wall, J. Munding, and A. M. Rey, Phys. Rev. Lett. **117**, 195302 (2016).
- [20] T. Lepers, D. Davesne, S. Chiacchiera, and M. Urban, Phys. Rev. A **82**, 023609 (2010).
- [21] K. O’Hara, S. Hemmer, M. Gehm, S. Granade, and J. E. Thomas, Science **298**, 2179 (2002).
